# Supplementary material for: An Optimization Framework to Enforce Multi-View Consistency for Texturing 3D Meshes
Source: arXiv:2403.15559 source file (2024-08-02)
Supplement: Supplementary file 1 [file 08_suppl.tex]

\newpage

\centerline{\Large Supplementary Material}

\setcounter{page}{1}
\section{Details in Stage I}
\subsection{Multi-View Consistent Initialization}
We utilize the multi-view depth-conditioned albedo diffusion model from RichDreamer
~\cite{richdreamer} for the initialization. The rendered depth maps are concatenated with the latent features to serve as input for the UNet denoiser~\cite{Ramesh_Pavlov_Goh_Gray_Voss_Radford_Chen_Sutskever_2021}. We only sample 8 images around the underlying 3D model instead of an overcomplete set, and we unproject all images to get an averaged RGB UV map as initialization. The invisible regions on the UV map are extracted by pixel detection and inpainted~\cite{Telea_2004} by the region neighborhood. The inpainted UV map is then decoded to latent space and noised to the specified diffusion step. Although the sampled images have fewer details and are averaged in UV space, this is sufficient for initialization~\cite{Meng_Song_Song_Wu_Zhu_Ermon_2021}.

\subsection{Defects in Latent UV Mapping}
\Cref{Figure:latent-uv-error} illustrates why details are dropped during the aggregation step when using latent UV map. Each pixel of the latent image represents a patch (e.g., $8\times8$) of the original image. Latent pixels warping means patches warping on RGB space, which inevitably leads to blurring or jagged lines after decoding.
\begin{figure*}[h]
\centering
\setlength{\tabcolsep}{2.5pt}
\includegraphics[width=0.9\textwidth]{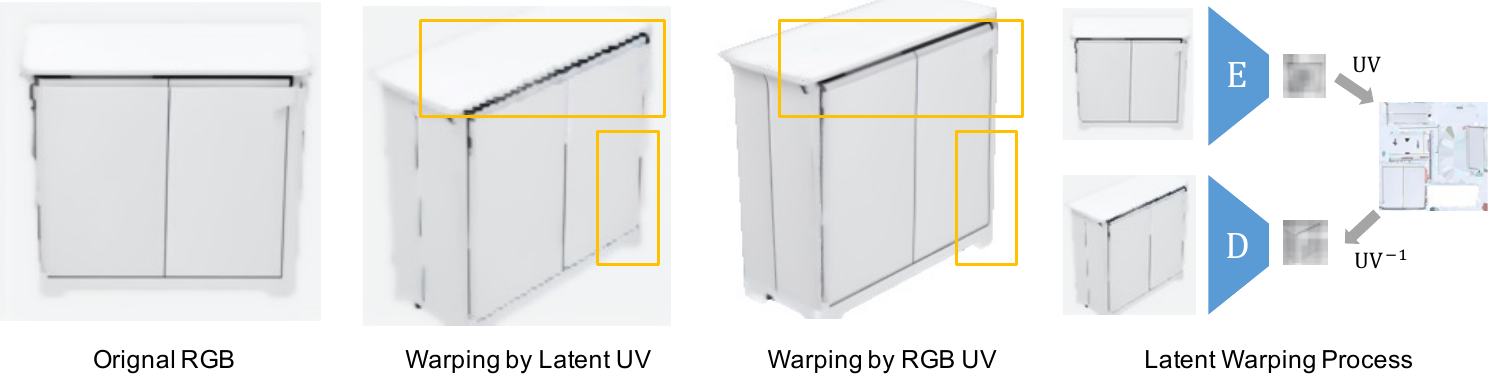}
\caption{\small{The left image is the original RGB image. The second column is the warping image caused by latent UV. The third column is the warping image by RGB UV. Using RGB UV warping, everything is in good order. Using latent UV warping, the straight horizontal line becomes a set of horizontal line segments, and the details are blurred.
}}

\label{Figure:latent-uv-error}
\end{figure*}
\section{Texture Stitching details}

In this section, we provide details on the formulations of $\phi_f(z_f)$ and $\phi_{ff'}(z_f, z_{f'})$.

\noindent\textbf{Formulation of $\phi_f(z_f)$.} With $\set{C}_{f,i} = \{\bs{c}\}$ we denote all colors of pixels of image $I_i$ associated with face $f$. Let $\set{C}_{f} = \cup_{1\leq i \leq k}$ collect all the colors of the pixels associated with the face $f$. We perform mean sift clustering among $\set{C}_f$. With $\bs{c}_f$ and $\sigma_f$ we denote the center of the cluster and the associated variance, respectively. We then define 
\begin{equation}
\phi_f(z_f) = \left\{
\begin{array}{cc}
+\infty & \set{C}_{f,z_f} = \emptyset \\
\frac{1}{\set{C}_{f,z_f}}\sum\limits_{\bs{c}\in \set{C}_{f,z_f}}\frac{\|\bs{c}-\bs{c}_f\|^2}{2\sigma_f^2}&\textup{otherwise}
\end{array}
\right.\ .
\end{equation}

\noindent\textbf{Formulation of $\phi_{ff'}(z_f, z_{f'})$.} Denote $\set{P}_{f,i}$ as the set of pixels in $I_i$ that belong to face $f$. If $\set{P}_{f,i}\neq \emptyset$, we compute $\bs{f}_{f,i} = (\overline{\bs{c}}_{f,i},\mu \overline{\bs{d}}^{\SIFT}_{f,i}$, where $\overline{\bs{c}}_{f,i}$ is the average pixel color among $\set{P}_{f,i}$ and $\overline{\bs{d}}^{\SIFT}_{f,i})$ is the average SIFT pixel descriptor among $\set{P}_{f,i}$. We set $\mu = 1$ in this paper. Note that instead of merely using color differences, we observe that incorporating SIFT helps place cuts among textureless regions. 

Our definition of $\phi_{ff'}(z_f, z_{f'})$ differs from that of ~\cite{DBLP:conf/eccv/WaechterMG14} in the sense that we take advantage of the consistency of the images, in contrast to simply using color differences. Specifically,
\begin{itemize}
\item When $\set{P}_{f,z_f} =\emptyset$ or $\set{P}_{f',z_{f'}} =\emptyset$, 
\begin{equation}
\phi_{ff'}(z_f, z_{f'}) =+\infty.
\label{Eq:Color:Difference0}
\end{equation}
\item When $\set{P}_{f,z_{f'}} =\emptyset$ and $\set{P}_{f',z_{f}} =\emptyset$, 
\begin{equation}
\phi_{ff'}(z_f, z_{f'}) = \|\bs{f}_{f,z_f} - \bs{f}_{f',z_{f'}}\|^2.
\label{Eq:Color:Difference}
\end{equation}
\item When $\set{P}_{f,z_{f'}} \neq \emptyset$ and $\set{P}_{f',z_{f}} =\emptyset$,
\begin{equation}
\phi_{ff'}(z_f, z_{f'}) = \|\bs{f}_{f,z_f} - \bs{f}_{f,z_{f'}}\|^2.
\label{Eq:Color:Difference1}
\end{equation}
\item When $\set{P}_{f,z_{f'}} = \emptyset$ and $\set{P}_{f',z_{f}} \neq \emptyset$,
\begin{equation}
\phi_{ff'}(z_f, z_{f'}) = \|\bs{f}_{f,z_f} - \bs{f}_{f',z_{f}}\|^2.
\label{Eq:Color:Difference2}
\end{equation}
\item When $\set{P}_{f,z_{f'}} \neq \emptyset$ and $\set{P}_{f',z_{f}} \neq \emptyset$,
\begin{equation}
\phi_{ff'}(z_f, z_{f'}) = \frac{1}{2}\Big(\|\bs{f}_{f,z_f} - \bs{f}_{f',z_{f}}\|^2+\|\bs{f}_{f,z_f} - \bs{f}_{f,z_{f'}}\|^2\Big).
\label{Eq:Color:Difference3}
\end{equation}
\end{itemize}

Note that we only compute the color difference in \cref{Eq:Color:Difference} when $z_f$ and $z_{f'}$ are not available in either $f$ or $f'$. 
Otherwise, we employ the color consistency in \cref{Eq:Color:Difference1,Eq:Color:Difference2,Eq:Color:Difference3} which better reveals the appearance continuity after stitching.

\section{Visualization of Ablation Study}
\Cref{fig:ablation study} is a visualization of ablation study. The green box in “No alternating optimization” indicates that the inconsistency issues were partly resolved during view selection and alignment stages.

\begin{figure}
\begin{center}
   \includegraphics[width=0.9\textwidth]{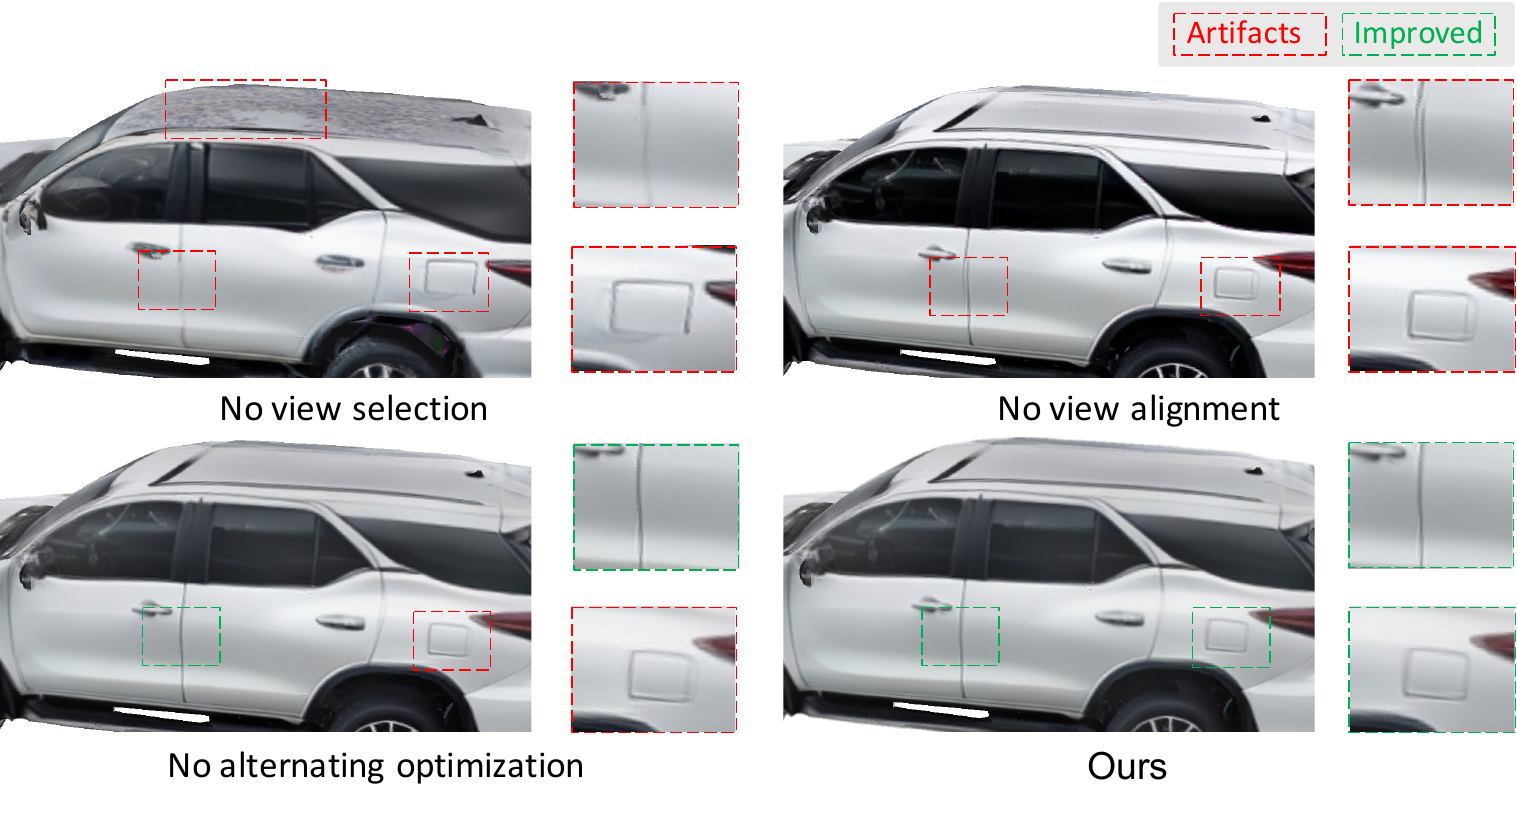}
   \caption{Visualization of Ablation Study}
\label{fig:ablation study}
\end{center}
\end{figure}

\section{Additional Results}

\subsection{Additional Baselines}
The latest non-open source methods TexFusion~\cite{Cao_2023_ICCV} and Decorate3D~\cite{decorate3d} are compared with our method in \cref{fig:Comparison_TexFusion} and \cref{fig:Comparison_Decorate3D}, from where we see that our results are more natural in color and have clearer details.

\begin{center}
\centering
\captionsetup{type=figure}
\includegraphics[width=1.0\textwidth]{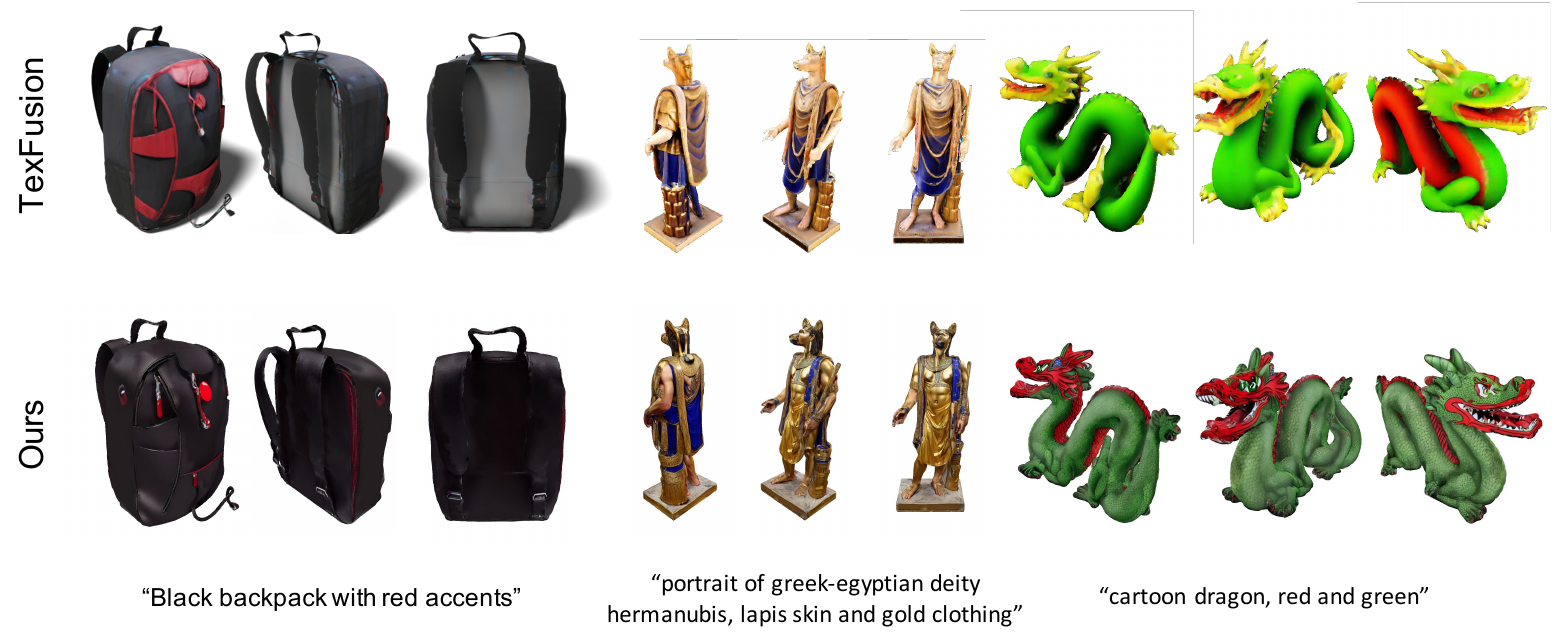}
\captionof{figure}{ Qualitative comparison with TexFusion: clearer details.}
\label{fig:Comparison_TexFusion}
\end{center}

\begin{center}
\centering
\captionsetup{type=figure}
\includegraphics[width=1.0\textwidth]{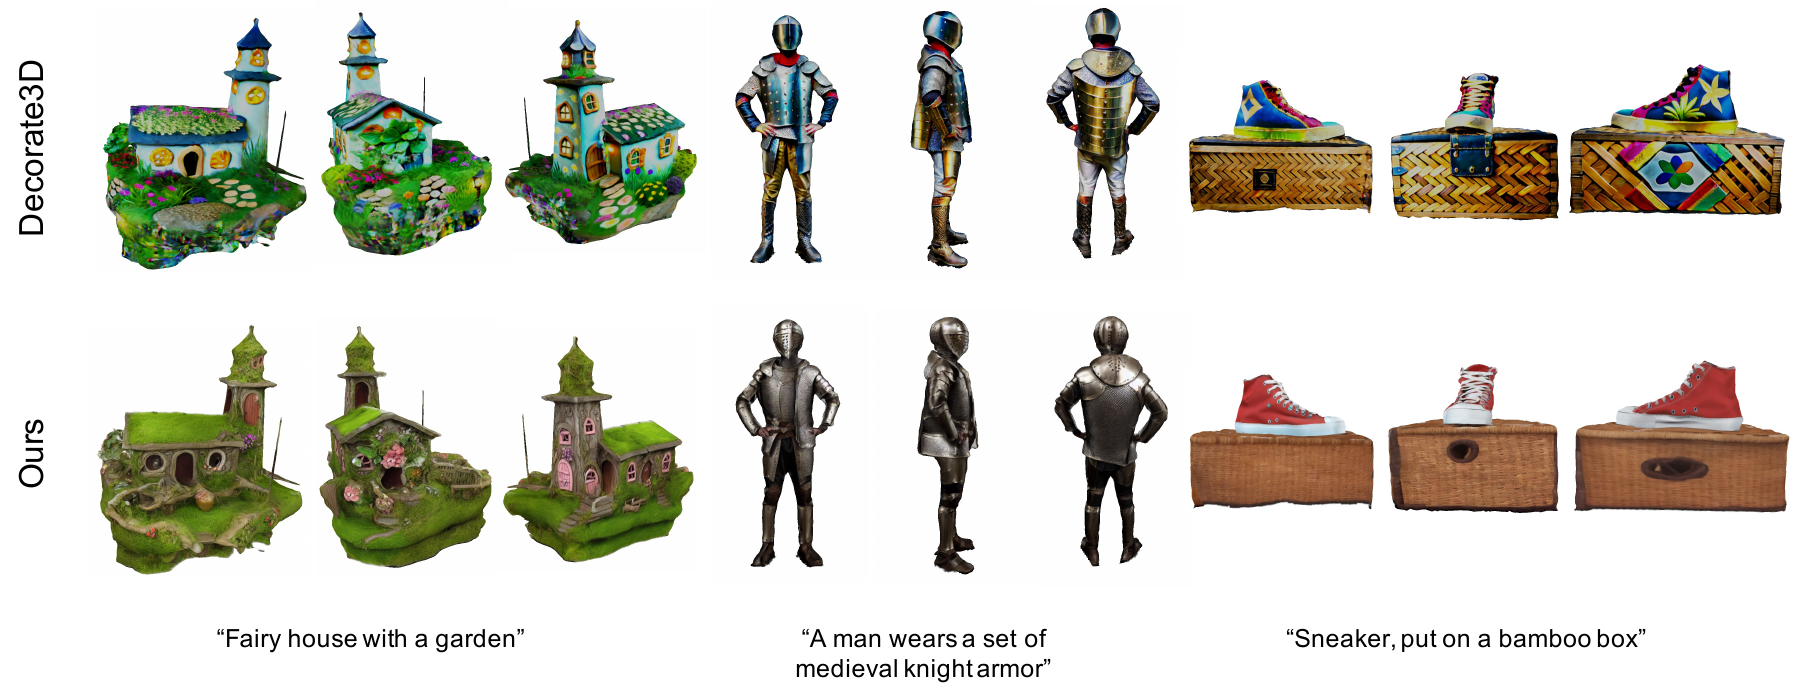}
\captionof{figure}{Qualitative comparison with Decorate3D: more natural in color.}
\label{fig:Comparison_Decorate3D}
\end{center}

\subsection{More Visual Results}
\Cref{fig:more_results:multiprompts} shows the results of different prompts on the same mesh.
We present more visual results on 25 objects from different categories in GObjaverse dataset~\cite{richdreamer} in \cref{fig:more_results:part0,fig:more_results:part1,fig:more_results:part2}. 
Each textured mesh is rendered to 8 views. A full list of object indexes and prompts can be found in \cref{table:model_source}.

\begin{center}
\centering
\captionsetup{type=figure}
\includegraphics[width=1.0\textwidth]{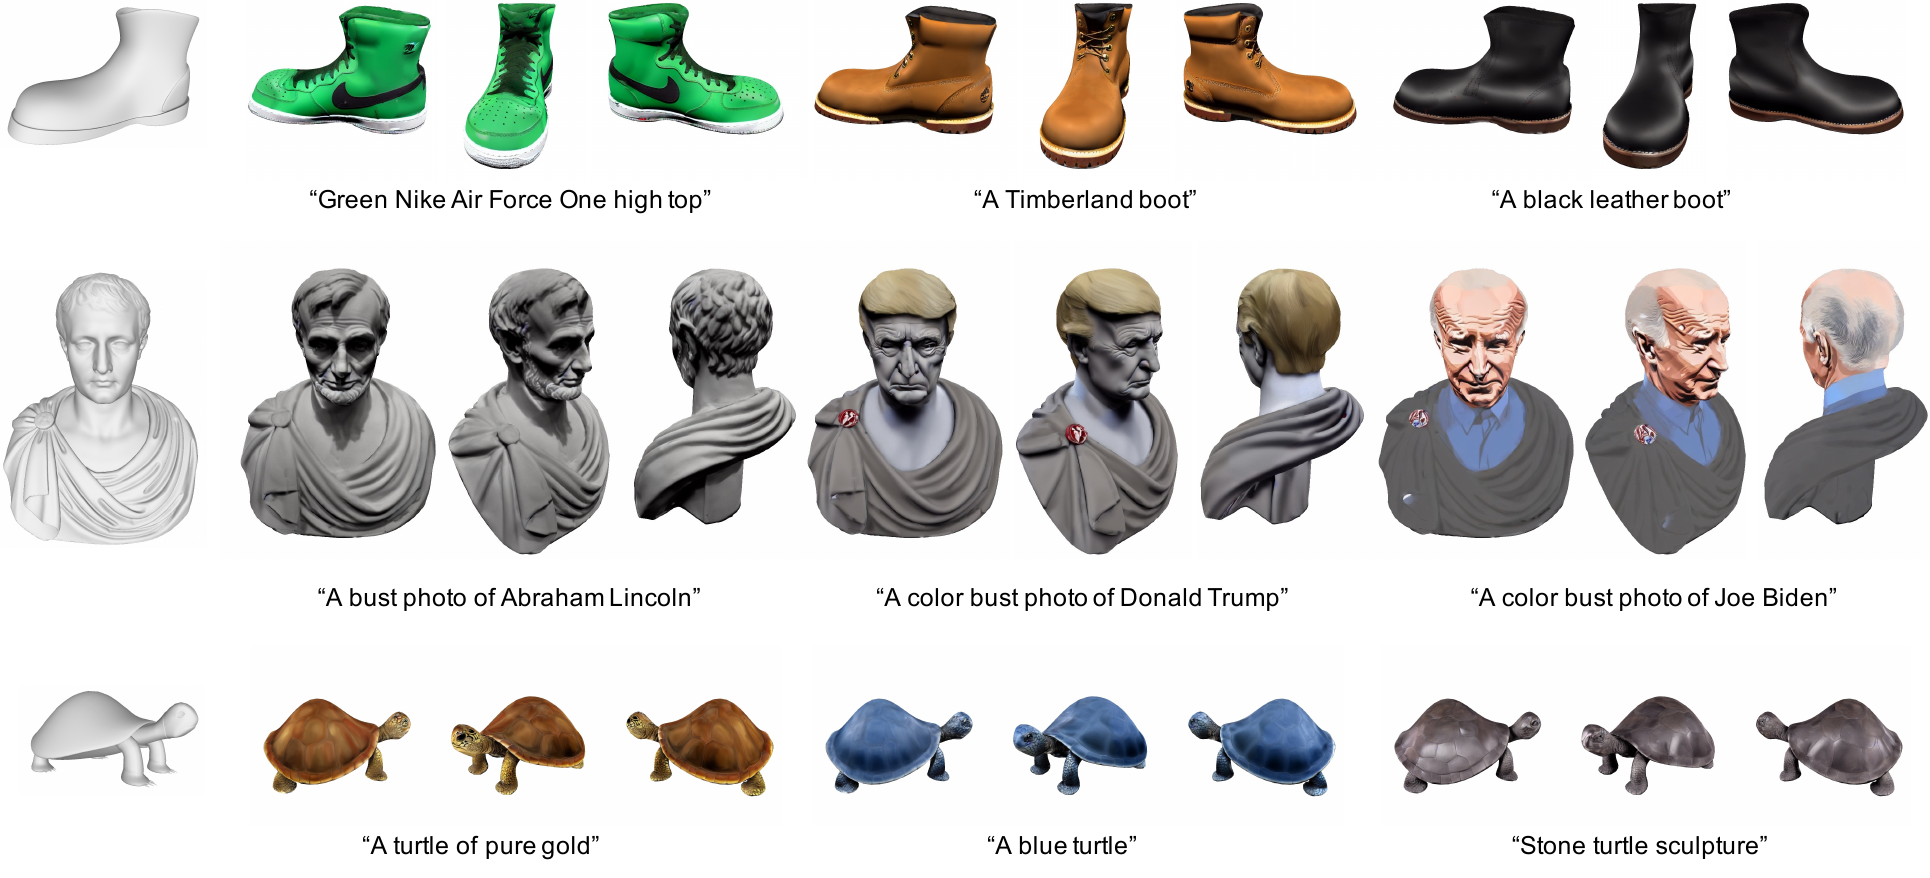}
\captionof{figure}{Different prompts for the same mesh.}
\label{fig:more_results:multiprompts}
\end{center}

\begin{center}
\centering
\captionsetup{type=figure}
\includegraphics[width=1.0\textwidth]{}
\includegraphics[width=1.0\textwidth]{}

\captionof{figure}{Gallery of textured meshes.}
\label{fig:more_results:part0}
\end{center}

\begin{center}
\centering
\captionsetup{type=figure}

\includegraphics[width=1.0\textwidth]{}
\includegraphics[width=1.0\textwidth]{}
\includegraphics[width=1.0\textwidth]{}
\includegraphics[width=1.0\textwidth]{}
\includegraphics[width=1.0\textwidth]{}
\includegraphics[width=1.0\textwidth]{}
\includegraphics[width=1.0\textwidth]{}
\includegraphics[width=1.0\textwidth]{}
\includegraphics[width=1.0\textwidth]{}
\includegraphics[width=1.0\textwidth]{}
\includegraphics[width=1.0\textwidth]{}
\includegraphics[width=1.0\textwidth]{}

\captionof{figure}{Gallery of textured meshes.}
\label{fig:more_results:part1}
\end{center}

\begin{center}
\centering
\captionsetup{type=figure}
\includegraphics[width=1.0\textwidth]{}
\includegraphics[width=1.0\textwidth]{}
\includegraphics[width=1.0\textwidth]{}
\includegraphics[width=1.0\textwidth]{}
\includegraphics[width=1.0\textwidth]{}
\includegraphics[width=1.0\textwidth]{}
\includegraphics[width=1.0\textwidth]{}
\includegraphics[width=1.0\textwidth]{}
\includegraphics[width=1.0\textwidth]{}
\includegraphics[width=1.0\textwidth]{}
\includegraphics[width=1.0\textwidth]{}

\captionof{figure}{Gallery of textured meshes.}

\label{fig:more_results:part2}
\end{center}

\begin{table}[b]
\caption{The object indexes and the corresponding text prompts.}
\centering
\resizebox{1.0\textwidth}{!}{
    \begin{tabular}{cc}
    
\toprule 
\textbf {Object Index} & \textbf{Prompt} \\ 

\midrule
0002c6eafa154e8bb08ebafb715a8d46 & Birthday cake \\
\midrule
000f88bb21164319ae797d315be6bc0e & Watch Model With Stand \\
\midrule
0023717f4f564cc99f4ded70db04f590 & Rusty kerosene lamp \\
\midrule
0023b3edbc114be188ca9d8f729dfaaf & a vintage car \\
\midrule
0025c5e2333949feb1db259d4ff08dbe & A wooden bird house \\
\midrule
00286954e2d54db8bc7832cc8682b6ff & Furniture Bed \\
\midrule
002e02c30121465c8a01bcb83b584ea5 & A pair of blue jeans \\
\midrule
003199cc6ff2410cb2d8e6f8a9cbb163 & a Portugal Fire Hydrant \\
\midrule
0032696f5871429fbd0549d9628f812c & A Christmas present \\
\midrule
0033322379a24798a6875a5cb2de54f5 & A raspberry \\
\midrule
0046f208ef8d4988ba7bb9d297f29ec7 & An old Dutch windmill building \\
\midrule
004fb4d72f6c4e55a15b9025a868d1a3 & a roast chicken \\
\midrule
0056880681c044cb9fe815a9eed0425d & A rhino \\
\midrule
00602ef508784e5384665aacaaf1f3a0 & A handle saw \\
\midrule
0064add4992b426cb2f862e5875ebf6d & A pink donut \\
\midrule
0083fa5f10a442408e0f3f88df19c8ad & An ancient shield \\
\midrule
0087dc01648d4cc792a7d1e49848b825 & Stone horse head sculpture \\
\midrule
00978a128283411582590096643ec101 & A pale yellow seahorse \\
\midrule
00b267b43669422cbb4ec3a4e9b1c16e & A pair of sunglasses \\
\midrule
00d56831f9bc49f9a668f418c1af7558 & A dancing brown dog in a white shirt, wearing dark sunglasses \\
\midrule
010b9ece8a3a49e3b73be0b3cd02c720 & A brown vase with red roses \\
\midrule
011f2cd821e94596863378daa134cf0e & An Apple computer monitor \\
\midrule
013c3a1d945a4336a87f889c3d4c25b1 & Precision Sniper Rifle, CSGO AWP DRAGON LORE \\
\midrule
015777939fc3429ba4b5343be9d51ffa & A kid's bike \\
\midrule
017fe235577b4083ab32c2b7949ba022 & A platinum ring studded with precious stones \\

\bottomrule

    \end{tabular}}
   
    \label{table:model_source}
\end{table}
